# Supplementary material for: DoGE: Domain Reweighting with Generalization Estimation
Source: arXiv:2310.15393 source file (2024-02-05)
Supplement: Supplementary file 1 [file appendix.tex]

\appendix

\section{\textcolor{myred}{Derivation from Online Mirror Descent with Bregman Divergent Constraint}}\label{apd:derivation}

\paragraph{Universal Generalization.}
 To realize the optimal \emph{universal generalization} ability within $\mathcal{T}$ steps, we optimize $\alpha_t$ at each training step $t$, which minimizes averaged cross-entropy loss $\Bar{L}(\vtheta_{T})$ across all $k$ domains at the final stage. 
 Denote $l(\vtheta)$ as the next-token prediction (cross-entropy) loss of model parameterized by $\vtheta$, $l_i(\vtheta)$ as the loss of the $i^{th}$ domain $D_i$, our final objective can be written as:
\begin{align}\label{apd-equ:obj-T}
    \min_{\alpha_1, \hdots, \alpha_T \in \Delta^{k-1}} \Bar{L}(\theta_{T}) = \min_{\alpha_1, \hdots, \alpha_T \in \Delta^{k-1}} \sum_{i \in [k]} l_i(\theta_{T})
\end{align}

With a greedy approximation of~\eqref{apd-equ:obj-T}, we search for the optimal domain weights $\alpha_t$ to minimize the average loss over $k$ domains at step (t+1):

\begin{align}\label{apd-equ:obj-t0}
    \argmin_{\alpha_t \in \Delta^{k-1}} \Bar{l}(\theta_{t+1}) &= \argmin_{\alpha_t\in \Delta^{k-1}} \sum_{i \in [k]} l_i(\theta_{t+1}) \notag\\
                                                      &= \argmin_{\alpha_t\in \Delta^{k-1}} \sum_{i \in [k]} [l_i(\theta_{t+1}) - l_i(\theta_{t})]
\end{align}
Take the first-order approximation, we estimate the loss for $i^{th}$ domain as: 
\begin{align}
    l_i(\theta_{t+1}) &= l_i(\theta_{t}) + \nabla l_i(\theta_{t}) \cdot (\theta_{t+1} -\theta_{t}) + O(\|\theta_{t+1} - \theta_{t+1}\|^2) \notag \\
                      &\approx l_i(\theta_{t}) + \nabla l_i(\theta_{t}) \cdot \left[ -\eta_t \cdot \sum_{j\in [k]} \alpha_T^j \nabla l_j(\theta_{t})\right] \notag \\
\end{align}

Denote $\Grad_t^i := \nabla l_i(\theta_{t})$, $\Wt^i := \nabla l_i(\theta_{t}) \cdot \left[ \sum_{j\in [k]} p_t^j \nabla l_j(\theta_{t})\right]$, \eqref{apd-equ:obj-t0} can be written as:
\begin{align}\label{apd-equ:obj-t1}
    \min_{\alpha_t \in \Delta^{k}} \Bar{l}(\theta_{t+1}) &= \min_{\alpha_t\in \Delta^{k}} \eta_t \cdot\sum_{i \in [k]} l_i(\theta_{t+1}) \notag\\
                                                      &\approx \min_{\alpha_t\in \Delta^{k-1}} -\eta_t \cdot\sum_{i \in [k]}\Grad_t^i \left( \sum_{j \in [k]} \alpha_t^j\Grad_t^j \right) \notag\\
                                                      &= \min_{\alpha_t\in \Delta^{k-1}} -\eta_t \cdot\sum_{i \in [k]} \alpha_t^i \left(\Grad_t^i \sum_{j \in [k]}\Grad_t^j \right) \notag\\
                                                      &= \min_{\alpha_t\in \Delta^{k-1}} -\eta_t \cdot\sum_{i \in [k]} \alpha_t^i \Wt^i \notag\\
                                                      &= \min_{\alpha_t\in \Delta^{k-1}} -\eta_t \cdot \langle \alpha_t, \Wt \rangle
\end{align}

For the sake of stability, we introduce a regularization term via Bregman divergence $D_h(\alpha || \alpha_{t-1}) = h(\alpha) - h(\alpha_{t-1}) - \langle \nabla h(\alpha_{t-1}), \alpha - \alpha_{t-1} \rangle$, $h(\alpha) = \sum_i \alpha_i \ln \alpha_i$. Adding this to \eqref{apd-equ:obj-t1}, our optimization problem is:

\begin{align}\label{apd-equ:obj-t}
    \alpha_t &:= \argmin_{\alpha \in \Delta^{k-1}} \Bar{l}(\theta_{t+1}) \notag\\
        &\approx \argmin_{\alpha \in \Delta^{k-1}} - \eta_t \cdot \langle \alpha, \Wt \rangle + \mu\cdot D_h(\alpha || \alpha_{t-1}) \notag\\
        &= \argmin_{\alpha \in \Delta^{k-1}} - \eta_t \cdot\langle \alpha, \Wt \rangle + \mu (h(\alpha) - \langle \nabla h(\alpha_{t-1}), \alpha\rangle)
\end{align}

With $\nabla h(\alpha) =  [\ln \alpha^i + 1]_i$, we take derivative of \eqref{apd-equ:obj-t}:
\begin{align}\label{apd-equ:derivative-t}
    \nabla(\cdot) &= \nabla\left(- \eta_t \cdot \langle \alpha, \Wt \rangle + \mu (h(\alpha) - \langle \nabla h(\alpha_{t-1}), \alpha\rangle)\right) \notag\\
                  &= -\eta_t \cdot\Wt + \mu[\ln \alpha + 1]_i - \mu[\ln \alpha_{t-1} + 1]_i = 0
\end{align}

\begin{equation}
    \Rightarrow \ln \alpha_t := \ln \alpha_* = \ln \alpha_{t-1} + \displaystyle{\frac{\eta_t \Wt}{\mu}}
\end{equation}

\paragraph{Generalization to a subset of target domains. ($D_{eval}\subset D_{train}$)}
Here we derive the update rule if we only target at a subset of domains $D_{eval}\subset D_{train}$:

\begin{align}
    \min_{\alpha_1, \hdots, \alpha_T \in \Delta^{k-1}} \Bar{L}(\theta_{T}) = \min_{\alpha_1, \hdots, \alpha_T \in \Delta^{k-1}} \sum_{i \in [D_{eval}]} l_i(\theta_{T})
\end{align}

Denote $\Grad_t^i := \nabla l_i(\theta_{t})$, we search for the optimal domain weights $\alpha_t$ to minimize the average loss over $D_{eval}$ at step (t+1):

\begin{align}\label{apd-equ:obj-t0}
    \argmin_{\alpha_t \in \Delta^{k-1}} \sum_{i \in [D_{eval}]} l_i(\theta_{t+1}) &= \argmin_{\alpha_t\in \Delta^{k-1}} \sum_{i \in [D_{eval}]} l_i(\theta_{t+1}) \notag\\
                                                      &= \argmin_{\alpha_t\in \Delta^{k-1}} \sum_{i \in [D_{eval}]} [l_i(\theta_{t+1}) - l_i(\theta_{t})] \notag\\
                                                      &= \argmin_{\alpha_t\in \Delta^{k-1}} -\eta_t \cdot\sum_{i \in [k]} \alpha_t^i \left(\Grad_t^i \sum_{i \in [D_{eval}]}\Grad_t^j \right) 
\end{align}

Alternatively, we define the generalization gain of $i^{th}$ domain for the targeted evaluation domains $D_{eval}$ as $\Wt_{eval}^i := \nabla l_i(\theta_{t}) \cdot \left[ \sum_{j\in [D_{eval}]} \alpha_t^j \nabla l_j(\theta_{t})\right]$. Therefore, the optimization problem can be written as:

\begin{align}
    \argmin_{\alpha_t \in \Delta^{k-1}} \sum_{i \in [D_{eval}]} l_i(\theta_{t+1}) &= \argmin_{\alpha_t\in \Delta^{k-1}} -\eta_t \cdot\sum_{i \in [k]} \alpha_t^i \left(\Grad_t^i \sum_{i \in [D_{eval}]}\Grad_t^j \right)  \notag\\
                                                      &= \argmin_{\alpha_t\in \Delta^{k-1}} -\eta_t \cdot\sum_{i \in [k]} \alpha_t^i \Wt_{eval}^i \notag\\
                                                      &= \min_{\alpha_t\in \Delta^{k-1}} -\eta_t \cdot \langle \alpha_t, \Wt_{eval} \rangle
\end{align}

With Bregman divergence $D_h(\alpha || \alpha_{t-1}) = h(\alpha) - h(\alpha_{t-1}) - \langle \nabla h(\alpha_{t-1}), \alpha - \alpha_{t-1} \rangle$, $h(\alpha) = \sum_i \alpha_i \ln \alpha_i$, we can derive the update rule \ref{apd-equ:update_dw_eval}

\begin{align}
    \alpha_t &:= \argmin_{\alpha \in \Delta^{k-1}} \sum_{i \in [D_{eval}]} l_i(\theta_{t+1}) \notag\\
        &\approx \argmin_{\alpha \in \Delta^{k-1}} - \eta_t \cdot \langle \alpha, \Wt_{eval} \rangle + \mu\cdot D_h(\alpha || \alpha_{t-1}) \notag\\
        &= \argmin_{\alpha \in \Delta^{k-1}} - \eta_t \cdot\langle \alpha, \Wt_{eval} \rangle + \mu (h(\alpha) - \langle \nabla h(\alpha_{t-1}), \alpha\rangle)
\end{align}

\begin{equation}\label{apd-equ:update_dw_eval}
    \Rightarrow \ln \alpha_t^i := \ln \alpha_*^i = \ln \alpha_{t-1}^i + \displaystyle{\frac{\eta_t \Wt_{eval}}{\mu}}
\end{equation}

\section{Interpretation of Generalization Estimation Function.}\label{apd:interpretation}
With the ultimate goal to improve pretrained model's generalization ability, the assumption underlies our algorithm is that \textbf{\emph{the domains are supposed to be up-weighed if it trains the model to generalize better to all the other domains}}. Following~\cite{pruthi2020tracin}, we estimate the generalization gain on a target domain $\mathcal{D}_{tgt}$ from a source domain $\mathcal{D}_{src}$ by decomposing the loss reduction along the training trajectory on all samples from other domains. 
Consider the model $\mathcal{M}$ parameterized with $\theta_t$ at step $t$. By training on sample $z_{src} \in \mathcal{D}_{src}$, the model is updated from $\theta_t$ to $\theta_{t+1}$. We estimate the point-wise generalization gain at $(t+1)$ step $\mathcal{W}_{t}(\cdot, z_{tgt})$ upon $z_{tgt} \in \mathcal{D}_{tgt}$ with the loss reduction $\mathcal{W}_{t}(\cdot, z_{tgt})=l(\theta_t, z_{tgt})-l(\theta_{t+1}, z_{tgt})$. Assume the step-wise update of the model is small, we apply the first order taylor expansion at $\theta=\theta_t$,  
\begin{equation}\label{apd-equ:delta-loss}
    l(\theta_{t+1}, z_{tgt}) = l(\theta_{t}, z_{tgt}) + \nabla l(\theta_{t}, z_{tgt}) \cdot (\theta_{t+1} -\theta_{t}) + O(\|\theta_{t+1} - \theta_{t+1}\|^2)
\end{equation}

If the model is optimized with stochastic gradient descent (SGD), the parameter update $(\theta_{t+1} -\theta_{t})$ equals to the stochastic gradient at $\theta_t$. We use it to approximate the update from other optimizers (AdamW, AdaGrad) for computational feasibility. Plug it in Equ. \ref{apd-equ:delta-loss}, the point-wise generalization gain can be estimated by the gradient multiplication on samples $z_{src}, z_{tgt}$:
\begin{align}\label{apd-equ:pointwise-gain}
    \mathcal{W}_{t}(z_{src}, z_{tgt}) &=l(\theta_t, z_{tgt})-l(\theta_{t+1}, z_{tgt})\notag\\
                               &\approx \displaystyle{-\nabla l(\theta_{t}, z_{tgt}) \cdot (\theta_{t+1} -\theta_{t})}\notag\\
                               &\approx \displaystyle{\eta_t \nabla l(\theta_{t}, z_{tgt}) \cdot \nabla l(\theta_{t}, z_{src})}\notag\\
                               &\propto \displaystyle{\nabla l(\theta_{t}, z_{tgt}) \cdot \nabla l(\theta_{t}, z_{src})}
\end{align}

Summing up the sample-wise gains across source/target domains' minibatches $(B_{src}, B_{tgt})$ according to Equ. \eqref{apd-equ:pointwise-gain}, the generalization gain on $B_{tgt}$ from training on $B_{src}$ can be derived as:
\begin{align}
    \mathcal{W}_{t}(B_{src}, B_{tgt}) &=\sum_{z_{tgt} \in B_{tgt}} l(\theta_t, z_{tgt})-l(\theta_{t+1}, z_{tgt})\notag\\
                               &\approx \sum_{z_{tgt} \in B_{tgt}} -\nabla l(\theta_{t}, z_{tgt}) \cdot (\theta_{t+1} -\theta_{t})\notag\\
                               &\propto \sum_{z_{tgt} \in B_{tgt}} \left(\sum_{z_{src} \in B_{src}} \nabla l(\theta_{t}, z_{tgt})\right) \cdot \nabla l(\theta_{t}, z_{src})
\end{align}

We finally arrive at the generalization estimation on $i^{th}$ domain at step $t$ as the overall generalization gain on the other $(k-1)$ domains. Denote the sampled mini-batches on each domain as $\{B_1, B_2, ..., B_k\}$, we estimate the utility of $i^{th}$ domain on generalization improvement of model $\theta_t$ as the overall generalization gain on $B_{tgt}=\bigcup_{j\in \{1, \cdots, k\}, j\neq i} B_j$ from training on $B_{src}=B_i$,

\begin{align}\label{apd-equ:generalization-gain}
    \mathcal{W}_{t}(D_i) &\approx \sum_{j\in \{1, \cdots, k\}, j\neq i} \mathcal{W}_{t}(B_i, B_j)\notag \\
                         &\propto \left(\sum_{j\in \{1, \cdots, k\}, j\neq i} \nabla l(\theta_{t}, B_j)\right) \cdot \nabla l(\theta_{t}, B_{i})
\end{align}

\section{Parameter Pruning}\label{apd:pruning}
We conduct parameter pruning by discarding the parameter-groups suffered from high cancellation effect (\eqref{equ:cancellation}) following Algorithm~\ref{alg:pruning}. We apply layer-pruning by setting parameters from each decoder-layer as one parameter-group and preserve 3 decoder-layers with lowest cancellation effect. Besides, we also experiment with more fine-grained pruning by setting each module-layer as one parameter-group and preserve 10 parameter-matrix with lowest cancellation effect.

\begin{algorithm*}[tb!]
   \caption{\doge Parameter-Pruning }
   \label{alg:pruning}
\begin{algorithmic}[1]
   \State {\bfseries Input:} Domain data splits $D_1,\dots, D_k$, cancellation-proxy model $\Mc(\vtheta)$, set of parameter-groups $\Sw$, number of selected parameter groups $k$, cancellation training steps $T_c$, batch size $b$ and step size $\eta_t$). 
   \vspace{2pt}
   \State Initialize cancellation-proxy model weights $\vtheta_0$
   \State Initialize cancellation scores for all parameter groups $\vw \in \Sw$ as 0:\\
        \vspace{4pt}
        \hspace{40pt} \emph{Score Dict} $R[\vw] \leftarrow 0.0$
   \vspace{2pt}
   
   \For{$t \in [T_c]$}
   \vspace{3pt}
        \State Uniformly sample minibatch $B_t=\{B_t^1,\dots,B_t^k\}$ of size $b$ 
        \vspace{3pt}
        \For{$\vw \in \Sw$}
            \State Obtain gradient for $\vw$: $||G(\vw)_t|| := \sum_{x_i \in B_t} \eta_t\| \displaystyle{\frac{\partial\ell(x_i)}{\partial \vw_t}}\|$
        \EndFor
        \State Update all model parameters $\vtheta \leftarrow \vtheta_{t+1}$
        \For{$\vw \in \Sw$}
            \State Obtain weight change: $\Delta \vw_t:=\| \vw_{t+1}-\vw_t \|$
            \State Compute cancellation at step $t$: $C_t(\vw) = \displaystyle{\frac{\|G(\vw)_t\|}{\| \vw_{t+1}-\vw_t \|}}$
            \State Update \emph{Score Dict} $R[\vw] \leftarrow R[\vw]+C_t(\vw)$
        \EndFor
   \EndFor
   \State \textbf{Return} Top-$k$ Parameter-groups $\{\vw_1, ..., \vw_k\}$  with lowest cancellation scores.
\end{algorithmic}
\end{algorithm*}

\section{Architecture of Models}
\begin{table}[htbp!]
\caption{Architecture hyperparameters for various model scales used in the paper. All models are vanilla Transformer decoder-only models.}
\label{tab:archictectures}
\centering
\vspace{5pt}
\begin{adjustbox}{max width=0.9\textwidth}
\begin{tabular}{lrrrrr}
\toprule
     & Layers & Attention heads & Attention head dim & Embed dim & Hidden dim \\
     \midrule
82M & 6      & 12               & 64                 & 768       & 3072       \\
124M & 12     & 12              & 64                 & 768       & 3072       \\
% 1.5B & 48     & 25              & 64                 & 1600      & 6400     \\  \bottomrule
\end{tabular}
\end{adjustbox}
\end{table}

\section{Details on the Evaluation Results}

\begin{table}[htbp!]
\vspace{-0.1in}
\caption{Domain Weights on SlimPajama-6B.}
\label{tab:dw-universal}
\centering
\begin{adjustbox}{max width=0.9\textwidth}
\begin{tabular}{lccc}
\toprule
                  & Baseline & DoReMi (82M) & \doge(82M)  \\ 
                  \midrule
Arxiv             & 0.166    &     0.097         &       0.058       \\
Book              & 0.166    &     0.156         &       0.029       \\
C4                & 0.166    &     0.146         &       0.039        \\
CommonCrawl       & 0.166    &     0.184         &       0.499       \\
Github            & 0.166    &     0.106         &        0.097      \\
StackExchange     & 0.166    &     0.112         &        0.114      \\
Wikipedia         & 0.166    &     0.198         &        0.165       \\
\bottomrule
\end{tabular}
\end{adjustbox}
\end{table}
